# Supplementary material for: NAP^2: A Benchmark for Naturalness and Privacy-Preserving Text Rewriting by Learning from Human
Source: arXiv:2406.03749 source file (2025-05-27)
Supplement: Supplementary file 1 [file sec_appendix.tex]

\section{Linguistic Quality Annotation}
\label{append:linguistic_quality}
% In this section, we provides the screenshot of our AMT task for privacy-aware text rewriting.

In this section, we demonstrate the questions that test the linguistic quality of the rewrites. The questions and annotation guidelines are listed follow,

\noindent \textbf{Q1}: How is the privacy protection degree of the rewritten sentence?
\begin{itemize}
    \item 3: The provided personal information cannot be inferred by the rewritten sentence at all. 
    \item 2: Hard to derive the personal information, but rewrite is weakly associated to the personal information. 
    \item 1: Part of the personal information can be inferred from the rewritten sentence. 
    \item 0: The personal information is fully contained in the rewritten sentence, directly or through paraphrasing.
\end{itemize}

\noindent \textbf{Q3}: How is the grammatical and fluency of the rewritten sentence?
\begin{itemize}
    \item 3: No grammatical error. 
    \item 2: Minor grammatical errors that do not affect understanding. 
    \item 1: Hard to derive the meaning but still a human language in English. 
    \item 0: Empty sentence or not english.
\end{itemize}

\noindent \textbf{Q2}: How is the semantic relevance of the rewritten sentence to the non-sensitive part of the original sentence? 
\begin{itemize}
    \item 3: Accurately preserves the meaning of the original sentence. 
    \item 2: Basically the same meaning but does not cover some minor content. 
    \item 1: Has a minor resemblance to the meaning of the original sentence, however, it is also misleading. 
    \item 0: Empty sentence or does not reflect the meaning of the original sentence at all.
\end{itemize}

\begin{table*}[t]
\centering
\begin{tabular}{l|cccccc}
\toprule
Model & P@1 & P@3 & P@5 & Rprec & NDCG & MAP \\
\midrule \midrule 
RANDOM$^\ddagger$ & 0.3333 & 0.3800 & 0.3560 & 0.3904 & 0.5775 & 0.4923 \\
\midrule
TOKEN MATCH$^\ddagger$ & 0.6533 & 0.4400 & 0.3120 & 0.4734 & 0.6507 & 0.5649 \\
BERT MATCH$^\ddagger$ & 0.7200 & 0.5889 & 0.4227 & 0.6864 & 0.7424 & 0.7261 \\ 
\midrule
% MEAN (RCE, $\alpha=0.0$) &  &  &  &  &  &  \\ 
MEAN ($\alpha=0.1$) & 0.7133 & 0.5800 & 0.4240 & 0.6822 & 0.7374 & 0.7202 \\ 
MEAN ($\alpha=0.2$)$^\ddagger$ & \textbf{0.7200} & \textbf{0.5889} & \textbf{0.4267} & \textbf{0.7044} & \textbf{0.7427} & \textbf{0.7279} \\ 
MEAN ($\alpha=0.3$) & 0.6933 & 0.5822 & 0.4253 & 0.6956 & 0.7346 & 0.7169 \\ 
% MEAN (RCE, $\alpha=0.4$) &  &  &  &  &  &  \\ 
\midrule
% OPT (RCE, $\alpha=0.0$) &  &  &  &  &  & \\ 
OPT ($\alpha=0.1$) & 0.7200 & 0.5867 & 0.4227 & 0.6942 & 0.7415 & 0.7254 \\ 
OPT ($\alpha=0.2$)$^\ddagger$ & 0.7200 & \textbf{0.5911} & \textbf{0.4267} & \textbf{0.7122} & 0.7440 & \textbf{0.7313} \\ 
OPT ($\alpha=0.3$) & \textbf{0.7333} & 0.5844 & \textbf{0.4267} & 0.7013 & \textbf{0.7450} & 0.7303 \\ 
OPT ($\alpha=0.4$) & 0.7200 & 0.5889 & 0.4240 & 0.7033 & 0.7429 & 0.7281 \\ 
\midrule
% LSAP (RCE, $\alpha=0.0$) &  &  &  &  &  &  \\
% LSAP (RCE, $\alpha=0.1$) & \textbf{0.7333} & 0.5933 & 0.4240 & 0.7011 & 0.7470 & 0.7331 \\
LSAP ($\alpha=0.2$) & 0.7267 & 0.6000 & 0.4267 & 0.7111 & 0.7469 & 0.7355 \\
LSAP ($\alpha=0.3$) & \textbf{0.7333} & \textbf{0.5933} & 0.4253 & 0.7078 & 0.7464 & 0.7331  \\
LSAP ($\alpha=0.4$)$^\ddagger$ & \textbf{0.7333} & 0.5911 & \textbf{0.4280} & \textbf{0.7156} & \textbf{0.7487} & \textbf{0.7373} \\
LSAP ($\alpha=0.5$) & 0.7133 & 0.5911 & 0.4267 & 0.7077 & 0.7437 & 0.7301 \\

%%% Test R0
% RANDOM & 0.3949 & 0.3897 & 0.3631 & 0.3955 & 0.6246 & 0.5234 \\
% \midrule
% TOKEN MATCH & 0.6821 & 0.4752 & 0.3385 & 0.5174 & 0.7009 & 0.6102 \\
% BERT & 0.7795 & 0.6205 & 0.4462 & 0.7195 & 0.7973 & 0.7700 \\ 
% \midrule
% % MEAN (RCE, $\alpha=0.0$) &  &  &  &  &  &  \\ 
% MEAN (RCE, $\alpha=0.1$) & 0.7692 & 0.6171 & 0.4503 & 0.7162 & 0.7953 & 0.7687 \\ 
% MEAN (RCE, $\alpha=0.2$) & 0.7641 & 0.6256 & 0.4533 & 0.7079 & 0.7924 & 0.7656 \\ 
% MEAN (RCE, $\alpha=0.3$) & 0.7744 & 0.6085 & 0.4462 & 0.7056 & 0.7908 & 0.7620 \\ 
% MEAN (RCE, $\alpha=0.4$) & 0.7385 & 0.5983 & 0.4400 & 0.6666 & 0.7741 & 0.7369 \\ 
% \midrule
% % OPT (RCE, $\alpha=0.0$) &  &  &  &  &  & \\ 
% OPT (RCE, $\alpha=0.1$) & 0.7795 & 0.6205 & 0.4492 & 0.7293 & 0.7979 & 0.7738 \\ 
% OPT (RCE, $\alpha=0.2$) & 0.7897 & 0.6274 & 0.4544 & 0.7395 & 0.8042 & 0.7828 \\ 
% OPT (RCE, $\alpha=0.3$) & 0.7590 & 0.6120 & 0.4410 & 0.7150 & 0.7894 & 0.7599  \\ 
% OPT (RCE, $\alpha=0.4$) & 0.7692 & 0.6154 & 0.4462 & 0.7129 & 0.7939 & 0.7673 \\ 
% \midrule
% % LSAP (RCE, $\alpha=0.0$) &  &  &  &  &  &  \\
% LSAP (RCE, $\alpha=0.1$) & 0.7897 & 0.6342 & 0.4523 & 0.7394 & 0.8059 & 0.7860 \\
% LSAP (RCE, $\alpha=0.2$) & 0.7795 & 0.6291 & 0.4513 & 0.7373 & 0.8009 & 0.7784 \\
% LSAP (RCE, $\alpha=0.3$) & 0.8154 & 0.6325 & 0.4533 & 0.7444 & 0.8116 & 0.7917 \\
% LSAP (RCE, $\alpha=0.4$) & 0.8000 & 0.6376 & 0.4533 & 0.7562 & 0.8082 & 0.7893 \\

\bottomrule
\end{tabular}
\caption{Experimental results of privacy leakage token detection using random guess (RANDOM), exact token match (TOKEN MATCH), BERT MATCH, and alignment models (MEAN, OPT and LSAP). The models with $\ddagger$ are selected and compared in our paper. }
\label{tab:privacy_detection_ir_all}
\vspace{-2mm}
\end{table*}

\section{Privacy Leakage Detection Experiments}
\label{append:privacy_detection_analysis}

\begin{table*}[h]
\centering
% \footnotesize
\begin{tabular}{l lll lll}
\toprule
& \multicolumn{3}{c}{Dev} & \multicolumn{3}{c}{Test}\\
\cmidrule(lr){2-4} \cmidrule(lr){5-7}
$\theta$ & P & R & F-1 & P & R & F-1\\
\midrule \midrule

0.40 & 64.62 & 88.79 & 74.80 & 55.60 & 88.94 & 68.46 \\
% 0.45 & 67.46 & 85.15 & 75.28 & 59.52 & 84.77 & 69.93 \\
0.50 & 72.73 & 82.12 & 77.14 & 64.49 & 82.06 & 72.22 \\
% 0.55 & 76.74 & 76.67 & 76.70 & 68.10 & 77.40 & 72.45 \\
0.60 & 81.12 & 70.00 & 75.15 & 72.56 & 69.29 & 70.89 \\
% 0.65 & 87.08 & 63.03 & 73.13 & 74.70 & 61.43 & 67.42 \\
0.70$^\ddagger$ & 92.31 & 54.55 & 68.57 & 77.31 & 49.14 & 60.09 \\
% 0.75 & 93.33 & 42.42 & 58.33 & 78.53 & 34.15 & 47.60 \\
0.80 & 99.05 & 31.52 & 47.82 & 87.61 & 24.32 & 38.08 \\
% 0.90 & 100.00 & 02.42 & 04.73 & 88.24 & 03.69 & 07.08 \\
\bottomrule
\end{tabular}
\caption{The comparison of privacy detection model using various thresholds $\theta \in [0.4, 0.8]$.}
\label{tab:privacy_detection_threhold}
% \vspace{-2mm}
\end{table*}

In Table~\ref{tab:privacy_detection_ir_all}, we demonstrate the full results of privacy leakage token detection using IR metrics. For alignment models, we search the margin hyper-parameter in $\{0.1, 0.2, 0.3, 0.4\}$. The model selected for each setting is noted with $\ddagger$.

In Table~\ref{tab:privacy_detection_threhold}, we illustrate the threshold selection process for our best detection model, i.e., LSAP ($\alpha=0.4$). With the increase of threshold $\theta$, precision increases and recall decreases. In our system, we target on a more reliable detection system and set $\theta=0.7$. Although the F1 score of $\theta=0.6$ is higher, we find the detection system tend to mask out useful information in the original sentence, which harms the performance in rewriting.

\begin{table*}[h]
\centering
\footnotesize
\begin{tabular}{l| cc cc | cc cc }
\toprule
& \multicolumn{4}{c|}{DELETE} & \multicolumn{4}{c}{OBSCURE}  \\
Model & BLEU & SARI & Sim$_s$ & Sim$_p$ &{} BLEU & SARI & Sim$_s$ & Sim$_p$\\
\midrule \midrule
COPY & 42.92 & 17.89 & 0.999 & 0.579 &{} 56.07 & 23.22 & 0.999 & 0.579\\
SEQ2SEQ & 09.50 & 28.00 & 0.492 & 0.438 &{} 08.41 & 24.33 & 0.544 & 0.476 \\
BackTrans & 15.80 & 30.76 & 0.739 & 0.573 &{} 18.07 & 25.89 & 0.739 & 0.573  \\
BART & 36.62 & 19.01 & 0.931 & 0.574 &{} 50.51 & 23.61 & 0.931 & 0.574 \\
Src & 42.46 & 31.03 & 0.927 & 0.581 &{} 40.26 & 35.68 & 0.885 & 0.576\\
Mask & 35.25 & 39.55 & 0.807 & 0.491 &{} 33.76 & 40.57 & 0.790 & 0.506 \\
Src+Persona & - & - & - & - &{} 31.75 & 35.35 & 0.819 & 0.710 \\
Mask+Persona & - & - & - & - &{} 27.58 & 37.55 & 0.774 & 0.695\\
% Src+Persona & 33.21 & 40.73 & 0.805 & 0.713 &{} 31.75 & 35.35 & 0.819 & 0.710 &{} 35.84 & 40.61 & 0.827 & 0.735 \\
% Mask+Persona & 28.50 & 40.32 & 0.774 & 0.688 &{} 27.58 & 37.55 & 0.774 & 0.695 &{} 31.21 & 40.66 & 0.778 & 0.711\\
\bottomrule

\end{tabular}
\caption{The comparison of rewriting models on DELETE, OBSCURE, using BLEU, SARI, semantic similarity (Sim$_s$) and persona similarity (Sim$_p$).}
\label{tab:generation_all}
\vspace{-2mm}
\end{table*}
\begin{table*}[h]
\small
\centering
\begin{tabular}{l| cccc }
\toprule
& \multicolumn{4}{c}{OBSCURE}\\
Model & BLEU & SARI & Sim$_s$ & Sim$_p$ \\
\midrule \midrule
% Src & 42.46 & 31.03 & 0.927 & 0.581 &{} 40.26 & 35.68 & 0.885 & 0.576 &{} 46.22 & 43.88 & 0.899 & 0.583\\

Src (w/o Constraint) &40.26 & 35.68 & 0.885 & 0.576 \\
\midrule
Src+Constraint($\lambda=1.25$) & 39.60 & 36.04 & 0.881 & 0.571 \\
Src+Constraint($\lambda=2.5$)$^\ddagger$ & 38.41 & 36.98  & 0.870 & 0.565\\
Src+Constraint($\lambda=5$) & 35.83 & \textbf{39.73} & 0.842 & 0.552\\
Src+Constraint($\lambda=10$) & 30.83 & 39.70 & 0.810 & 0.535 \\
\midrule \midrule
% Mask & 35.25 & 39.55 & 0.807 & 0.491 &{} 33.76 & 40.57 & 0.790 & 0.506 &{} 37.94 & 44.34 & 0.792 & 0.504\\

Mask (w/o Constraint) & 33.76 & 40.57 & 0.790 & 0.506 \\
\midrule
Mask+Constraint($\lambda=1.25$) & 33.33 & 40.56 & 0.790 & 0.506 \\
Mask+Constraint($\lambda=2.5$)$^\ddagger$ & 32.63 & \textbf{40.69} & 0.791 & 0.506 \\
Mask+Constraint($\lambda=5$) & 30.65 & 40.45 & 0.782 & 0.507\\
Mask+Constraint($\lambda=10$) & 26.51 & 39.86 & 0.767 & 0.501 \\
\bottomrule

\end{tabular}
\caption{Hyper-parameter selection for generation models with strategy-specific constraints in decoding.}
\label{tab:generation_constraint}
\vspace{-2mm}
\end{table*}

\section{Rewriting Experiments}
\label{append:rewriting_experiment}
In this section, we compare the rewriting models, in Table~\ref{tab:generation_all}. We find that BLEU only rewards correctly kept and inserted tokens, while falls to capture the removed tokens, which are essential in privacy-aware rewriting task. Therefore, BLEU is not included in our paper for comparison.
The hyper-parameter selection for knowledge constraint models are illustrated in Table~\ref{tab:generation_constraint}. Introducing strategy-specific knowledge constraints improves the performance of those models using whole original sentences as inputs, while do not help much on systems with masked inputs. We attribute this to the fact that Mask models have already eliminate the sensitive tokens and could not recover relevant expressions without corresponding inputs.
In order to have a consistent comparison, we choose $\lambda_u=\lambda_d=2.5$ in our paper.

\section{Knowledge Constraint Analysis}
\label{append:knowledge_constraint}

\begin{table*}[h]
\centering
\begin{tabular}{l|ccc|c}
\toprule
Relation Edge & Delete & Obscure & Steer & Selected\\
\midrule \midrule
RelatedTo & 14 & 147 & 103 & -\\
IsA & 1 & 100 & 31 & OBS \\
CapableOf & 4 & 47 & 23 & OBS\\
Synonym & 1 & 29 & 34 & -\\
UsedFor & 0 & 32 & 20 & -\\
Antonym & 1 & 11 & 41 & STE \\
DistinctFrom & 0 & 8 & 26 & STE\\
HasProperty & 1 & 4 & 16 & STE\\
AtLocation & 2 & 4 & 15 & STE\\
FormOf & 5 & 9 & 3 & -\\
HasPrerequisite & 1 & 10 & 5 & OBS\\
Desires & 2 & 11 & 3 & OBS\\
SimilarTo & 0 & 11 & 3 & OBS\\

\midrule

HasA & 0 & 7 & 4 & -\\
MotivatedByGoal & 2 & 3 & 2 & -\\
ReceivesAction & 0 & 6 & 2 & -\\
DerivedFrom & 0 & 6 & 0 & -\\
MannerOf & 0 & 4 & 1 & -\\
NotDesires & 0 & 4 & 1 & -\\
HasFirstSubevent & 0 & 1 & 2 & -\\
HasLastSubevent & 0 & 2 & 1 & -\\
InstanceOf & 0 & 3 & 0 & -\\
CausesDesire & 0 & 2 & 0 & -\\
PartOf & 2 & 0 & 0 & -\\
DefinedAs & 1 & 1 & 1 & -\\
HasSubevent & 1 & 1 & 0 & -\\
Causes & 1 & 1 & 1 & -\\
HasContext & 0 & 1 & 1 & -\\
EtymologicallyDerivedFrom & 0 & 1 & 0 & -\\
NotCapableOf & 0 & 1 & 0 & -\\
genre & 0 & 1 & 0 & -\\
EtymologicallyRelatedTo & 0 & 1 & 0 & -\\
\bottomrule
\end{tabular}
\caption{Correlation between knowledge constraints with a single relation type and rewriting strategies. The selected relation types for \textit{obscuring} and \textit{steering} are noted with OBS and STE.}
\label{tab:analyze_constraint_single_rel}
\vspace{-2mm}
\end{table*}

In Table~\ref{tab:analyze_constraint_single_rel}, we illustrate the statistic of tokens that are both in rewriting sentences and in neighbour of privacy-leakage tokens, distinguished by different relation types. We consider the relations i) with a total of more than 10 hits and ii) have a clear preference on a rewriting pattern (at least two times the number of the second highest pattern). We select \{\textit{IsA}, \textit{CapableO}, \textit{HasPrerequisite}, \textit{Desires} and \textit{SimilarTo}\} as constraints for OBSCURE, and \{\textit{Antonym}, \textit{DistinctFrom}, \textit{HasProperty},and \textit{AtLocation}\} as constraints for STEER.

\section{Private Information Alignment}
Given a message $x$ and a persona $p$, we construct a sentence level alignment score $A(x,p) \in [0, 1]$ defining the probability that message $x$ leaks persona $p$.

Given a dataset of conversations, where each conversation $C$ contains a set of sentences, and a set of utterances such that $C_i = \{X_i=\{x_1,x_2,...,x_m\}, P_i=\{p_1,p_2,...,p_n\}\}$, we
want to perform private information alignment to determine the probability that each utterance in a conversation is leaked by each utterance. For this, we can apply $A(x,p)$ to each sentence-utterance pair in a conversation. We can then use an information retrieval technique to determine which utterances are leaked by each sentence. We store this information and
use it in the Dataset Rewriting step to improve rewrite performance. We also use this information to define ground truths that are used later to evaluate the performance of both the Dataset Rewriting step and the Model Finetuning step.

For this study, three different alignment methods are evaluated.Those three methods are RoBERTa MNLI entailment scores, Sharp-MAX and Sparse-MAX scores. Each of these three methods outputs a probability that can be used as the alignment function $A(x,p) \in [0, 1]$. Then, the information retrieval technique is via naive thresholding, tuned on a test dataset. The three methods are evaluated on a test dataset of 100 pairs of utterances and personas, where utterance leaks persona $i$. We build a 100 x 100 matrix, where row $i$ represents utterance $i$ and column $j$ represents persona $j$. For each cell $i,j$ in the matrix, each of the three methods is used to output a probability. Then, different thresholds are tested to determine the best alignment method.

All algorithms produce sentence-wise alignment probabilities on a set of 200 utterance-persona pairs. Ideally, we want our algorithm to correctly pair each utterance with the persona it leaks, and none of the others. To do this, we threshold the probabilities with a static number, and say that probabilities below the threshold correspond to no alignment, and vice versa. A perfect algorithm would produce a perfect recall-precision=1.

In the analysis, we look to find an alignment solution which can maximise recall and precision. The strongest candidate is RoBERTa MNLI entailment. Different thresholds were examined, and ultimately a threshold of 0.3 was chosen with the recall is 0.69 and precision is 0.28. Figure \ref{fig:alighenment_LLM} display two different prompts that could be passed to an LLM. Alignment involves telling the model about private information next to the pieces of dialogue where the private information is mentioned.

\begin{table}[h]
\centering
\small
\begin{tabular}{l|c|cccc}
\toprule
Model & Set & Flu. & Sem. & Pri. & CPR(\%) \\ %
\midrule \midrule
 Src & DEL & 2.897 & 2.718 & 0.590 & 37.23\% \\ % r\_d\_S
 Mask & DEL & 2.407 & 2.272 & 1.889 & 53.08\% \\ % r\_d\_M
 \midrule
 Src & OBS & 2.614 & 2.506 & 1.016 & 66.33\% \\ % r\_o\_S
 Src+KC & OBS & 2.667 & 2.497 & 1.099 & 66.38\% \\ % r\_o\_S\_g
 Mask & OBS & 2.321 & 2.222 & 1.914 & 80.45\% \\ % r\_o\_M
 Mask+KC & OBS & 2.420 & 2.173 & 1.977 & 82.74\% \\ % r\_o\_M\_g
 \midrule 
 Src & STE & 2.341 & 2.183 & 1.524 & 74.37\% \\ % r\_s\_S
 Mask & STE & 2.439 & 2.246 & 2.118 & 73.90\% \\ % r\_s\_M
 Src+KC & STE & 2.500 & 2.493 & 1.832 & 76.83\% \\ % r\_s\_S\_g 
 Mask+KC & STE & 2.346 & 2.299 & 2.185 & 76.45\% \\ % r\_s\_M\_g
\bottomrule
\end{tabular}
\caption{The comparison of rewriting systemS using grammatical  fluency(Flu.),  semantic  relevance(Sem.)  and  privacy protection (Pri.) score and correct pattern rate (CPR).}
\label{tab:corpus_human_analysis}
\vspace{-2mm}
\end{table}
